# Supplementary material for: CbLDM: A Diffusion Model for recovering nanostructure from atomic pair distribution function
Source: arXiv:2509.01370 source file (2026-03-08)
Supplement: Supplementary file 1 [file supplementary.pdf]

## Supplementary

The following six figures are additional figures from section 4.2 of the article.

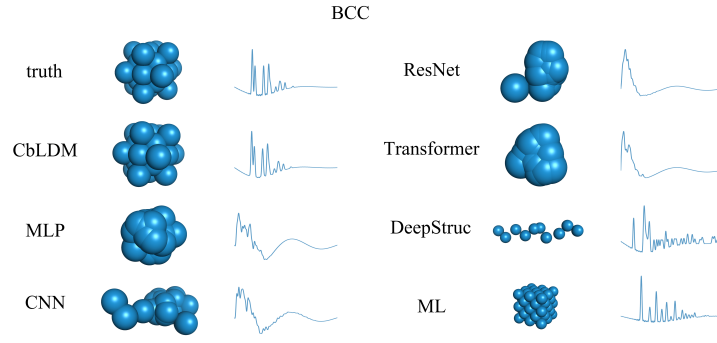

Figure 1: The prediction performance of CbLDM on the validation data of BCC structure.

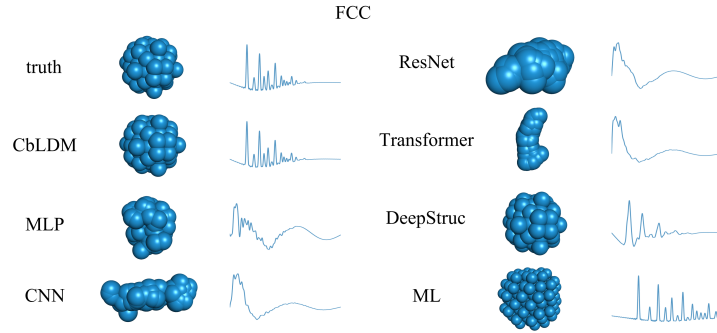

Figure 2: The prediction performance of CbLDM on the validation data of FCC structure.

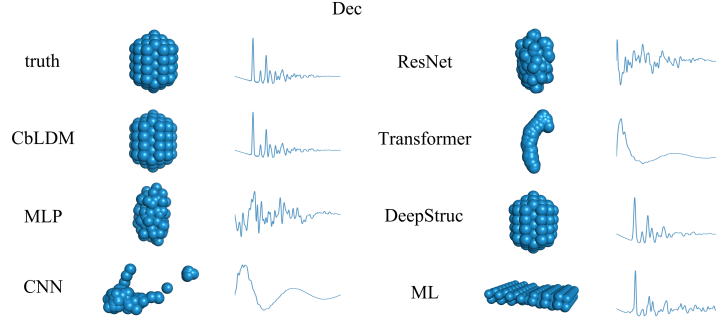

Figure 3: The prediction performance of CbLDM on the validation data of Dec structure.

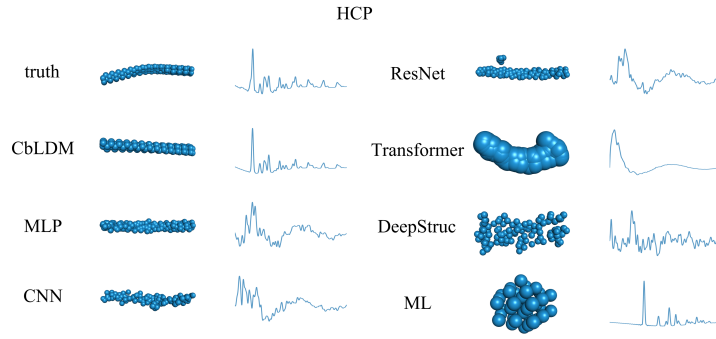

Figure 4: The prediction performance of CbLDM on the validation data of HCP structure.

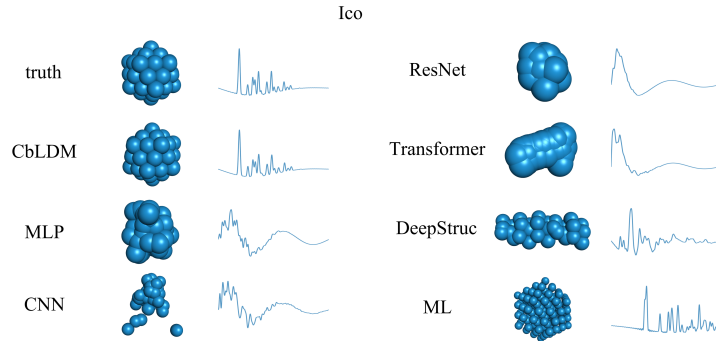

Figure 5: The prediction performance of CbLDM on the validation data of Ico structure.

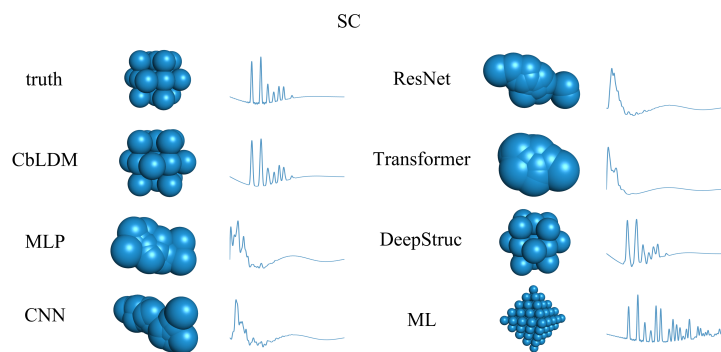

Figure 6: The prediction performance of CbLDM on the validation data of SC structure.
